# Supplementary material for: Neural Response Generation with Meta-Words
Source: arXiv:1906.06050 source file (2019-06-14)
Supplement: Supplementary file 1 [file appendix.tex]

\begin{CJK*}{UTF8}{gbsn} 
\end{CJK*}
